# Supplementary material for: Does Invariant Risk Minimization Capture Invariance?
Source: arXiv:2101.01134 ancillary file (2021-02-26)

```

In[12]:= (*Loss Functions*)
sqLs[zh_, z_] := 0.5 * (zh - z)^2;
logLs[zh_, z_] := Log[1 + Exp[-z * zh]];

(*Notation :
>l=lambda, e=single environment, envs=list of environments, ls=loss function;
>x=φ(1,1)=-φ(-1,-1), y=φ(1,-1)=-φ(-1,1), by symmetry*)

(*Assumption: ls[a,b] = ls[-a,-b]*)
IRMparts[e_, ls_] := (a = e[[1]]; b = e[[2]]);
p00 = (1 - a) * (1 - b); p01 = (1 - a) * b; p10 = a * (1 - b); p11 = a * b;
R = p00 * ls[x, 1] + p01 * ls[y, 1] + p10 * ls[-y, 1] + p11 * ls[-x, 1];
gradR = D[R /. {x → w * x, y → w * y}, w] /. {w → 1};
{R, gradR});

(*Solve IRM_S*)
IRMsInvariant [envs_, ls_] :=
  (gradConstraints = Function[e, IRMparts[e, ls][[2]] == 0] /@ envs;
  NSolve[gradConstraints, {x, y}, Reals]);
IRMsMin[envs_, ls_] := (Parts = Function[e, IRMparts[e, ls]] /@ envs;
  gradConstraints = Function[p, p[[2]] == 0] /@ Parts;
  objective = Sum[p[[1]], {p, Parts});
  optProb = Prepend[gradConstraints, objective];
  NMinimize[optProb, {x, y}]);

(*Solve IRMv1*)
IRMv1e[e_, l_, ls_] := (A = IRMparts[e, ls]; A[[1]] + l * (A[[2]])^2);
IRMv1[envs_, l_, ls_] := Sum[IRMv1e[e, l, ls], {e, envs}];
IRMv1StationaryPts [envs_, l_, ls_] := (loss = IRMv1[envs, l, ls];
  Dx = D[loss, x];
  Dy = D[loss, y];
  NSolve[Dx == 0 && Dy == 0, {x, y}, Reals]);
IRMv1GlobalMin [envs_, l_, ls_] := (Sols = IRMv1StationaryPts [envs, l, ls];
  minSol = First@Sort[Sols, (loss /. #1) < (loss /. #2) &];
  {loss /. minSol, minSol});
(*Remark: It was observed that NMinimize doesn't always give the Global Minimum;
That's why we do the above.*)

In[1]:= (*Plot properties*)
ImgPlot[z_] := Rasterize[Show[z, ImageSize → Large], "Image"];
thikk = 0.005;

```

```

In[46]:= (*----- PART 1: Case of Squared Loss (sqls) -----*)
(*Grad constraints w/ SqLoss : Environments in E_{0.1}*)
PlotGradConstraints [alpha_, betaList_, ls_, yrange_, xrange_] := (
  envs = Function[e, {alpha, e}] /@ betaList;
  Eqs = Function[e, IRMparts[e, ls][[2]]] /@ envs;
  ImgPlot[ContourPlot[Eqs, yrange, xrange,
    AspectRatio -> Automatic,
    PlotLegends -> Function[beta,
      Style[StringForm["e = (``,``)", alpha, beta], FontSize -> 16]] /@ betaList,
    ContourStyle -> {Thickness[thikk], Thickness[thikk], Thickness[thikk],
      Thickness[thikk]},
    LabelStyle -> Directive[FontSize -> 16]]];

```

```

alpha = 0.1;
betaList = {0.2, 0.25, 0.4, 0.9};
PlotGradConstraints [alpha, betaList, sqls, {y, -0.65, 1.05}, {x, -0.15, 1.05}]

```

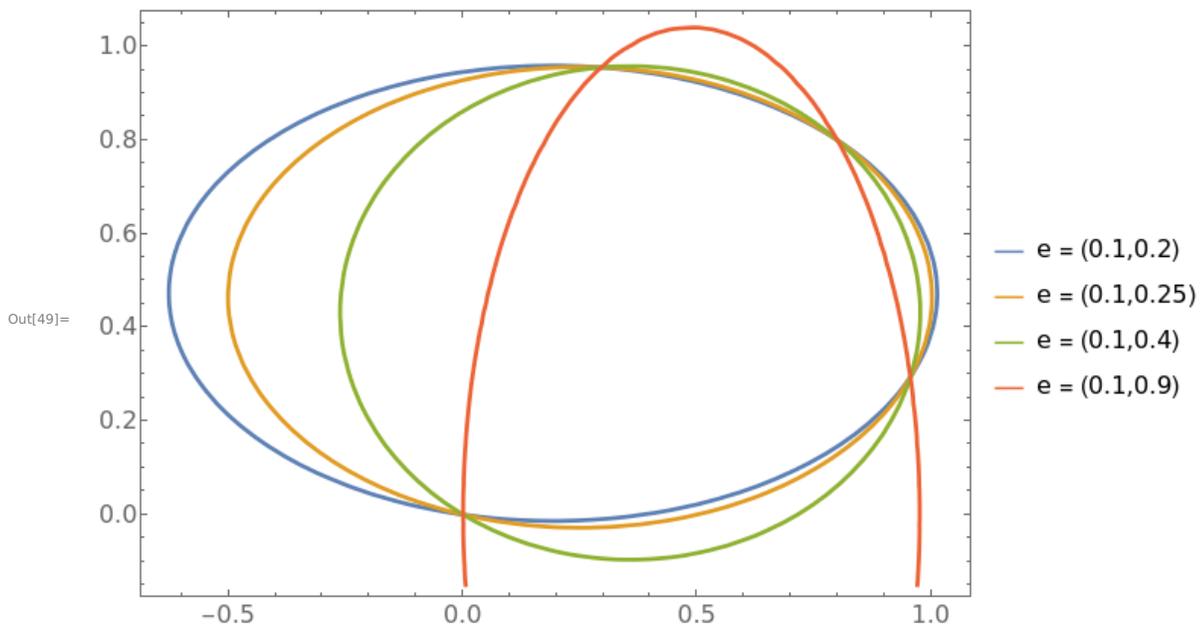

```

In[50]:= (*Loss of all predictors in I_S(E_alpha) across all E_alpha*)
LossVsEnvs[alpha_, sols_, ls_] := (
  betaList = Range[0, 1, 0.1];
  AllEnvs = Function[beta, {alpha, beta}]/@betaList;
  AllLosses[pt_] := Function[e, (IRMparts[e, ls][[1]] /. pt)]/@AllEnvs;
  BetaVsLoss[pt_] := Transpose @ {betaList, AllLosses[pt]};
  Plots = BetaVsLoss /@ Sols;
  ImgPlot[ListPlot[Plots,
    Joined -> {True, True, True, True},
    PlotRange -> All,
    PlotLegends ->
      Function[s, Style[s, FontSize -> 16]]/@ {"psi_IRM", "psi_1", "psi_2", "psi_0"},
    PlotStyle -> {Thickness[thikk], Thickness[thikk], Thickness[thikk], Thickness[thikk]},
    LabelStyle -> Directive[FontSize -> 16]]];

```

```

alpha = 0.1;
envs = {{alpha, 0.2}, {alpha, 0.3}};
Sols = IRMsInvariant[envs, sqls]
LossVsEnvs[alpha, Sols, sqls]

```

```

Out[53]= {{x -> 0.8, y -> 0.8}, {x -> 0.955719, y -> 0.294281},
  {x -> 0.294281, y -> 0.955719}, {x -> 0., y -> 0.}}

```

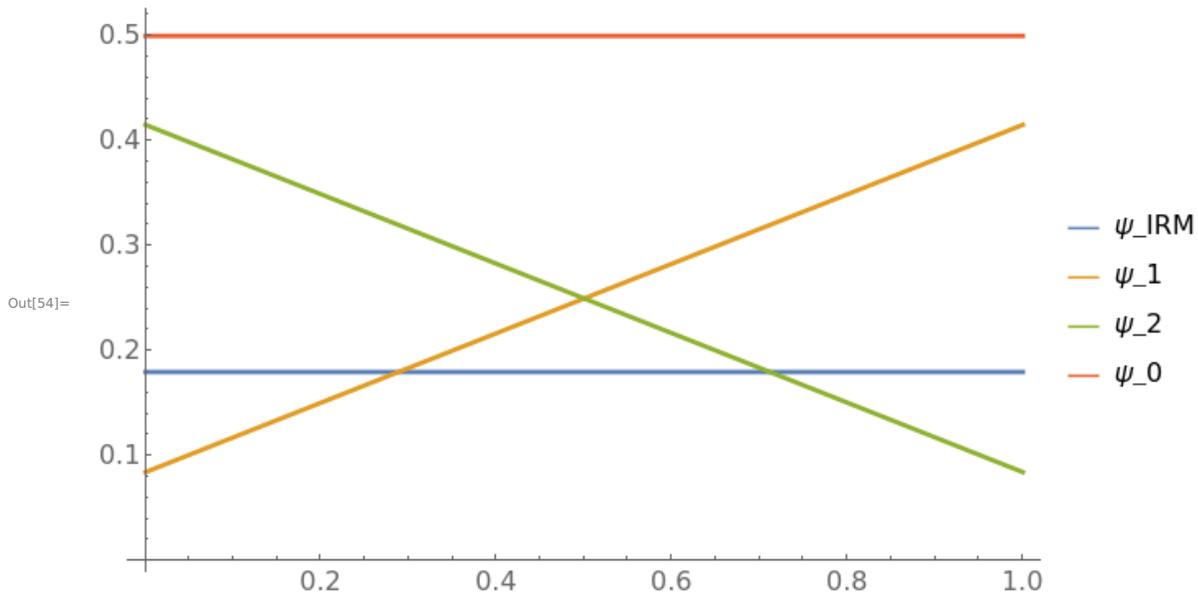

```

In[55]:= (*Solve IRMv1 for various choices of lambda;
Plot optimal predictor vs lambda*)
PlotIRMv1[envs_, ls_] := (
nonzerologlmbdalist = Range[0, 25];
loglmbdalist = Prepend[nonzerologlmbdalist, -1];
lmbdalist = Prepend[Function[x, 2^x]/@nonzerologlmbdalist, 0];
Solns = Function[l, IRMv1GlobalMin[envs, l, ls]]/@lmbdalist;
lmbdaSoln = Transpose@{loglmbdalist, Solns};
(*LambdaVsLs = Function[a,{a[[1]],a[[2]][[1]]}]@lmbdaSoln;
(*optional plot loss vs lambda*)*)
LmbdaVsX = Function[a, {a[[1]], Lookup[a[[2]][[2]], x]}]@lmbdaSoln;
LmbdaVsY = Function[a, {a[[1]], Lookup[a[[2]][[2]], y]}]@lmbdaSoln;
LmbdaVsmX = Function[a, {a[[1]], -Lookup[a[[2]][[2]], x]}]@lmbdaSoln;
LmbdaVsmY = Function[a, {a[[1]], -Lookup[a[[2]][[2]], y]}]@lmbdaSoln;
ImgPlot[ListPlot[{LmbdaVsX, LmbdaVsY, LmbdaVsmY, LmbdaVsmX},
Joined → {True, True, True, True},
PlotRange → All,
PlotLegends →
Function[s, Style[s, FontSize → 16]]@{"φ(1,1)", "φ(1,-1)", "φ(-1,1)", "φ(-1,-1)"},
PlotStyle → {Thickness[thikk], Thickness[thikk], Thickness[thikk], Thickness[thikk]},
LabelStyle → Directive[FontSize → 16]]];

```

```

In[56]:= (*Good case*)
PlotIRMv1[{0.25, 0.1}, {0.25, 0.2}, {0.25, 0.3}], sqls]

```

Out[56]=

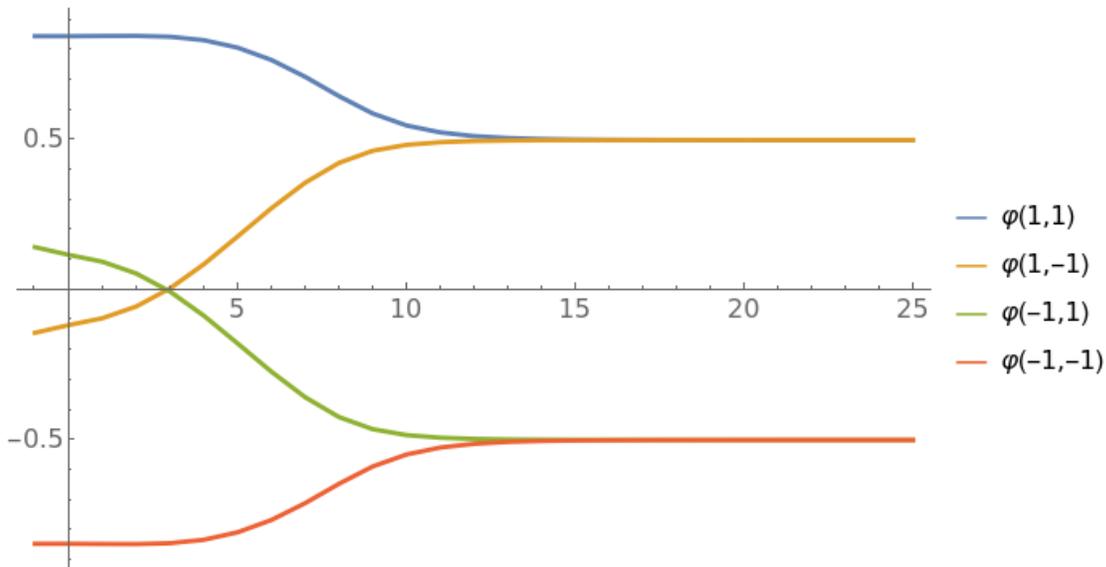

In[58]:= (\*Perturbed case\*)  
 PlotIRMv1[{{0.245, 0.105}, {0.255, 0.195}, {0.251, 0.302}}, sq]s]

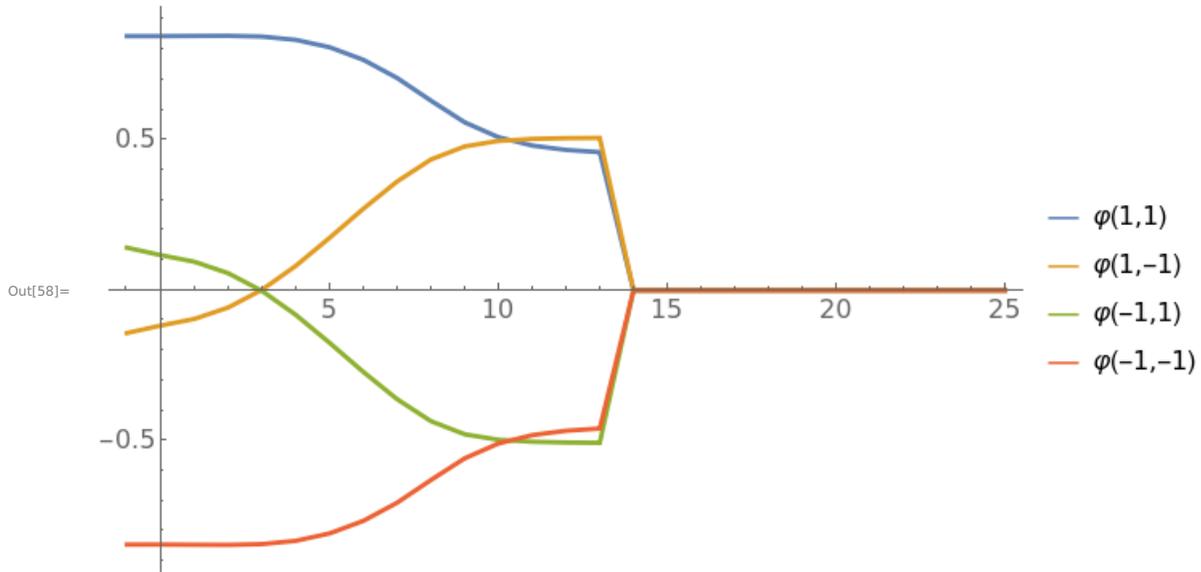

In[57]:= (\*Failure mode of IRM\_S\*)  
 PlotIRMv1[{{0.1, 0.2}, {0.1, 0.25}}, sq]s]

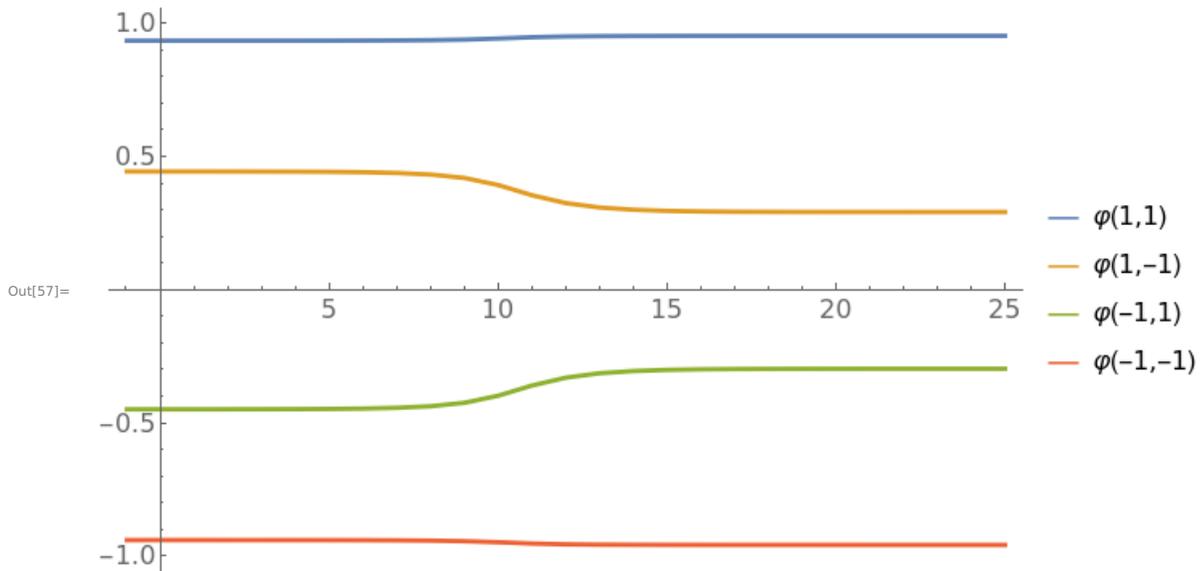

```
In[59]:= (*----- PART 2: Case of Logistic Loss (logls) -----*)
```

```
(*Grad constraints w/ LogLoss : Environments in E_{0.05}*)
```

```
alpha = 0.05;
```

```
betaList = {0.1, 0.2, 0.4, 0.9};
```

```
PlotGradConstraints [alpha, betaList, logls, {y, -2.75, 5.5}, {x, -2.75, 5.5}]
```

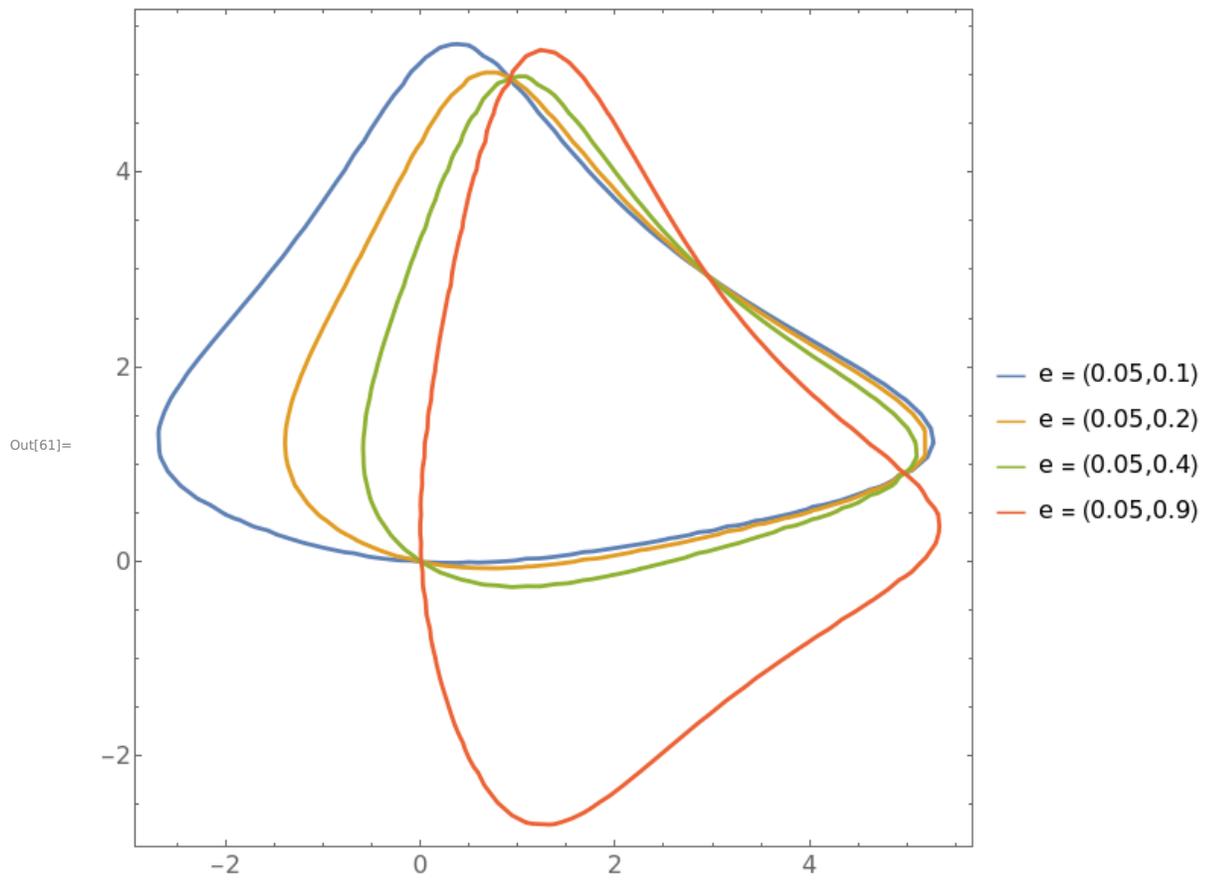

```

In[62]:= (*Unlike the case of sqls, Mathematica couldn't solve IRMsInvariant for logls;
we solved it numerically by zooming into plot above*)
alpha = 0.05;
betaList = {0.1, 0.2, 0.4, 0.9};
Sols = {{x -> 2.9444, y -> 2.9444},
        {x -> 4.9847, y -> 0.9041}, {x -> 0.9041, y -> 4.9847}, {x -> 0.0, y -> 0.0}};
gap = 0.0001;
Function[s,
(xr = {x, Lookup[s, x] - gap, Lookup[s, x] + gap};
yr = {y, Lookup[s, y] - gap, Lookup[s, y] + gap};
PlotGradConstraints [alpha, betaList, logls, yr, xr])/@ Sols

```

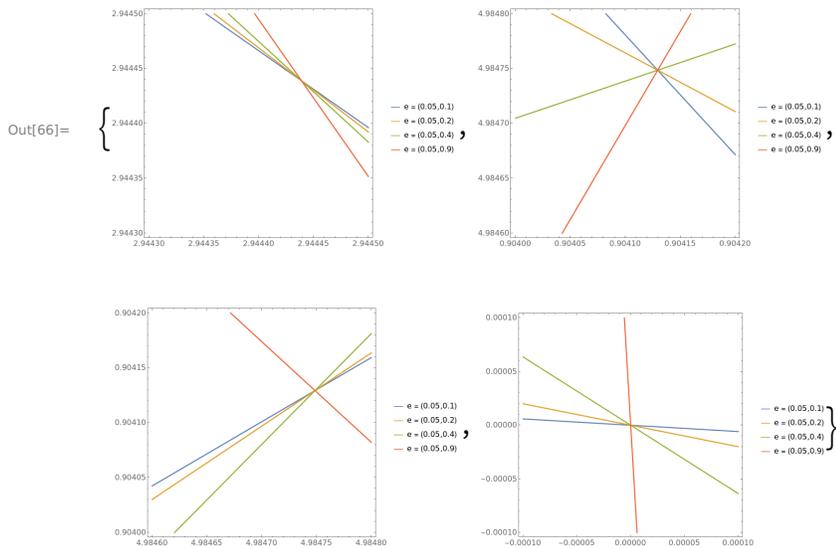

```
In[67]:= (*Loss of all predictors in I_S(E_alpha) across all E_alpha*)  
alpha = 0.05;  
Sols = {{x -> 2.9444, y -> 2.9444},  
        {x -> 4.9847, y -> 0.9041}, {x -> 0.9041, y -> 4.9847}, {x -> 0.0, y -> 0.0}}  
LossVsEnvs[alpha, Sols, logls]
```

```
Out[68]:= {{x -> 2.9444, y -> 2.9444}, {x -> 4.9847, y -> 0.9041},  
          {x -> 0.9041, y -> 4.9847}, {x -> 0., y -> 0.}}
```

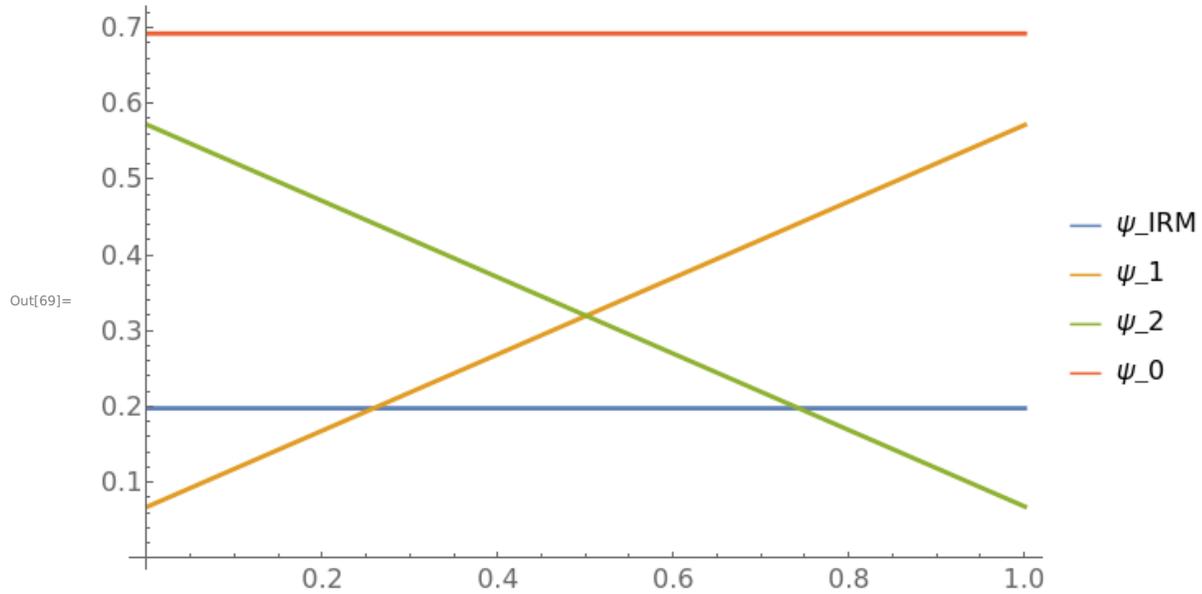

In[3]:= (\*---- PART 3: Losses when pure-IRM fails to pick the right predictor ----\*)

```

betaList = {-1/6, 1/3};
Loss1 = {1.41/3, 1.41/3};
Loss2 = {1.41/3 - 0.09 * 1/6, 1.5/3};
Loss0 = {0.5, 0.5};
Plots = Function[loss, Transpose @ {betaList, loss}] /@ {Loss1, Loss2, Loss0};
ImgPlot[ListPlot[Plots,
Joined -> {True, True, True},
PlotRange -> All,
PlotLegends -> Function[s, Style[s, FontSize -> 16]] /@ {"ψ_1", "ψ_2", "ψ_0"},
PlotStyle -> {Thickness[thikk], Thickness[thikk], Thickness[thikk]},
LabelStyle -> Directive[FontSize -> 16]]]

```

Out[8]=

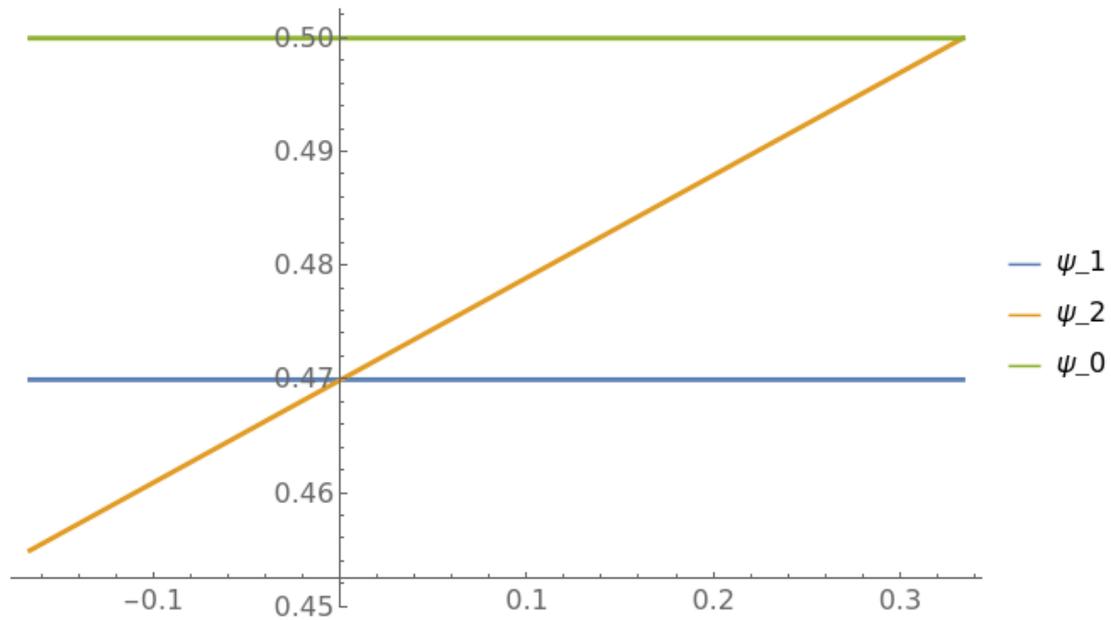

Supplement: Supplementary file 1 [file two-bit-irm.pdf]
